# Supplementary material for: KF-CS: Compressive Sensing on Kalman Filtered Residual
Source: arXiv:0912.1628 source file (2010-03-24)
Supplement: Supplementary file 2 [file appendix_kfcsstab_3.tex]

%\section{Appendix:  Proof of KF-CS Stability Result}
%\label{kfcs_stab_append}

\appendix

\subsection{Proof of  Theorem \ref{kfcs_stab}}
\label{append_kfcs}

%\subsubsection{Proof of Theorem \ref{kfcs_stab}}
%\label{kfcs_stab_proof}%is a direct consequence of the following lemmas. It
The proof follows by applying Lemma \ref{finitedelay} followed by Corollary \ref{kfinitwrong_cor} for each addition time.  %Lemma \ref{finitedelay} ensures that there are no false additions and computes the high probability detection delay $\tau_\dett$, under the assumption that all previous additions were detected. Lemma \ref{kfinitwrong} states that if the true support does not change after a certain time, and if it gets correctly detected by a certain time, $t_*$, KF-CS will converge to the genie-KF in mean-square and hence also in probability.% Corollary \ref{kfinitwrong_cor} (corollary of

\begin{lemma}
Under the assumptions of Theorem \ref{kfcs_stab},
\ben
\item there are no false additions, i.e. $\Nhat_t \subseteq N_t$
\item at each $t$, $\| x_t - \xhat_{t,\CSres}\|^2 \le B_*$
\item if at $t = t_{j}-1$, $\Nhat_t=N_t$, then w.p. $\ge (1-\eps)$,  $\Nhat_t = N_t$  for all $t \in [t_j + \tau_{\dett}(\eps,S), t_{j+1}-1]$.% all additions are detected, i.e
\een
\label{finitedelay}
\end{lemma}

The proof is given below in Appendix \ref{finitedelay_proof}.

The following lemma is similar to what should be a standard result for KF error convergence under wrong initial conditions, $\xhat_{t_*}, P_{t_*}$. Its proof should follow easily  from results in \cite{ekf}. Just for completion, we give its complete proof in Appendix \ref{kfinitwrongproof}. %(Added only for easy review).
\begin{lemma}
Assume that $x_t$ follows Signal Model \ref{randomwalk}. Also assume that for all $t \ge t_*$, $\Nhat_t = N_t = N_*$ and assume that $\delta_{|N_*|} < 1$. %The difference in the KF-CS and genie-KF estimates,
Then $\diff_t =\xhat_{t}-\xhat_{t,GAKF}$, converges to zero in mean square and hence also in probability. $\blacksquare$
\label{kfinitwrong}
\end{lemma}

A direct corollary of the above lemma is the following.
\begin{corollary}
Assume that $\Nhat_t = N_t = N_*$, for all $t \in [t_*, \ t_{**}]$. For a given $\eps, \eps_{\text{err}}$, there exists a $\tau_{KF}(\eps,\eps_{\text{err}},N_*)$ s.t. for all $t \in [t_* + \tau_{KF} , \ t_{**}]$, $Pr(\|\diff_t\|^2 \le \eps_{\text{err}}) > 1- \eps$. Clearly if $t_{**} < t_* + \tau_{KF}$, this is an empty interval.
\label{kfinitwrong_cor}
\end{corollary}

{\em Proof of Theorem \ref{kfcs_stab}: }
Define the event $E_j$ as $E_j:= \{ \Nhat_{t} = N_{t}, \forall \  t \in [t_j + \tau_{\dett}(\eps,S_a), t_{j+1}-1] \}$. Then Lemma \ref{finitedelay} implies that $Pr(E_{j}|E_1 \dots E_{j-1}) = Pr(E_{j}| E_{j-1}) \ge  1- \eps$. At the first addition time, $t_1=1$, we start with $N_{t_1-1} = N_0 = \Nhat_0$. Thus, from Lemma \ref{finitedelay}, $Pr(E_1) \ge 1-\eps$. Combining, these two facts, $Pr(E_j) \ge (1-\eps)^j$.%

Assume that $E_j$ occurs and apply Corollary \ref{kfinitwrong_cor} with $t_* =t_j + \tau_{\dett}(\eps,S_a)$ and $t_{**}= t_{j+1}-1$. Combining with  $Pr(E_j) \ge (1-\eps)^j$, the first claim follows.
%Then, there exists a $\tau_{KF}(\eps,\eps_{\text{err}},N_{t_j})$ s.t. for all $t \in  [t_j + \tau_{\dett}(\eps,S_a) + \tau_{KF}(\eps,\eps_{\text{err}},N_{t_j}), t_{j+1}-1]$, $Pr(\|\diff_t\|^2 \le \eps_{\text{err}} | A_j) > 1- \eps$. But $Pr(A_j) > (1-\eps)^j$. Thus $Pr(\|\diff_t\|^2 \le \eps_{\text{err}}) > (1-\eps)^{j+1}$. Since there are a maximum of $K$ addition times, $Pr(\|\diff_t\|^2 \le \eps_{\text{err}})  > (1-\eps)^{K+1}$.

The second and third claim are direct corollaries of Lemma \ref{finitedelay}. The last addition time is $t_K$. It is clear that if $E_1 \cap E_2 \dots \cap E_K$ occur, then all adds get detected before the next addition time and so at all times, $|\Delta| \le S_a$. The probability of this event is $(1-\eps)^K$. Since we have ensured zero false adds and our model assumes zero removals, $|\Delta_e|=0$ always. $\blacksquare$

\subsection{Proof of Lemma \ref{finitedelay}}%=x_t-\xhat_{t,\text{init}}
\label{finitedelay_proof}
The first two claims follow by induction. With  $\|w\|_\infty \le \lambda/\|A\|_1$, all results of \cite{dantzig} hold w.p. 1 (because eq 3.1  of \cite{dantzig} holds w.p. 1). From Theorem 1.1. of \cite{dantzig}, if a signal is $S$-sparse, and if $S \le \sinf$, then, its error after running the Dantzig selector is bounded by $B_*$.
At $t=0$, the first claim holds. So at $t=1$, $\beta_t$ will be $S_1 \le \smax$ sparse. Thus since $\smax \le \sinf$,  $\|\beta_t - \betahat_t\|^2 \le B_*$. But $x_t - \xhat_{t,\CSres} = \beta_t - \betahat_t$ and from this the second claim follows for $t=1$. This finishes the base case.
For the induction step, assume that the first two claims hold for $t-1$. Thus, at $t$, $\beta_t$ will be at most $S_t \le \smax$ sparse. Thus the second claim holds.
%Repeat the above argument to prove that the second claim holds for $t$. %Then $\beta_t=x_t-\xhat_{t,\text{init}}$ will be at most $\smax$ sparse. Thus since $\smax \le \sinf$,  $\|\beta_t - \betahat_t\|^2 \le B_*$. But $x_t - \xhat_{t,\CSres} = \beta_t - \betahat_t$ and from this the second claim will follow for $t$.
By setting the addition threshold $\alpha = B_*$, we ensure that for any $i$ with $x_i=0$, $(\xhat_{\CSres})_i^2 = (x_i - (\xhat_{\CSres})_i)^2 \le B_*=\alpha$ and from this the first claim follows for $t$.%it will never get falsely detected, . % and this gives the second claim This is the first claim.
%(A longer and clearer proof will follow by induction).

% given time
For the third claim, consider a newly added coefficient, $i$. It is easy to see (shown earlier) that if, at a $t$, $(x_t)_i^2 > 2 \alpha^2 + 2B_* = 4 B_*$, then $i$ will definitely get detected at $t$. Consider a $t \in [t_j, t_{j+1}-1]$. We have assumed that at $t = t_{j}-1$, $\Nhat_t=N_t$. Since the deletion step is not run, there cannot be false deletions and thus for any  $t \in [t_j, t_{j+1}-1]$, $|\Delta| \le S_a$. Consider the worst case:  no coefficient has got detected until  $t$, i.e. the current $\Delta=\add$ and so $|\Delta|=S_a$. All $i \in \Delta$ will definitely get detected at $t$ if $(x_t)_i^2 > 4B_*$ for all $i \in \Delta$. From our model, the different coefficients are independent, and for any $i \in \add$, $(x_t)_i^2 \sim \n(0, (t-t_j+1) \sigma_{sys}^2)$. Thus,
\bea
Pr((x_t)_i^2 > 4 B_*, \ \forall i \in \add) \se ( 2\Q(\sqrt\frac{4B_*}{(t-t_{j}+1) \sigma_{sys}^2}) )^{S_a} \nn
%\label{prxt}
\eea
%where $\Q(z):= \int_{z}^\infty (1/\sqrt{2\pi}) e^{-x^2/2} dx$ is the Gaussian Q-function.
Thus if if $t_j +\tau_{\dett} \le t_{j+1}-1$, then w.p. $\ge 1-\eps$, $\Nhat_t = N_t$ for all $t \in [t_j +\tau_{\dett}, t_{j+1}-1]$. This gives the third claim. $\blacksquare$%  $d > \tau_{\dett}(\eps,S_a)$, i.e.
% i.e. if $\add = \add(j)$ remains the same until $t_j +\tau_{\dett}$, then w.p. $\ge 1-\eps$, all current adds will get detected by $t_j +\tau_{\dett}$. Thus the third claim follows. $\blacksquare$%i.e. if no new additions occur for at least this much time,
